# Supplementary material for: Mixed-parity octupolar pairing and corner Majorana modes in three dimensions
Source: arXiv:2106.01361 ancillary file (2021-11-10)
Supplement: Supplementary file 1 [file Supplementary_OctupolPairing.pdf]

# Supplementary Material: Mixed-parity octupolar pairing and corner Majorana modes in three dimensions

Bitan Roy[1] and Vladimir Juričić[2,3]

[1]Department of Physics, Lehigh University, Bethlehem, Pennsylvania, 18015, USA
[2]Nordita, KTH Royal Institute of Technology and Stockholm University, Roslagstullsbacken 23, 10691 Stockholm, Sweden
[3]Departamento de Física, Universidad Técnica Federico Santa María, Casilla 110, Valparaíso, Chile

(Dated: November 2, 2021)

The Supplementary Material contains: (1) Band diagonalization of local pairing in octupolar Dirac insulator [see Sec. S1], (2) additional numerical results, showing evolution of topological superconductors [see Sec. S2], (3) parameter regime of the tight binding model over which the mixed parity octuplar pairings yield eight near zero energy Majorana corner modes [see Sec. S3], and (4) energy competition among all local pairings in an octupolar Dirac insulator [see Sec. S4].

## S1. BAND DIAGONALIZATION AND LOCAL OCTUPOLAR PAIRING IN DIRAC INSULATOR

In this section we show the band diagonalization procedure for an octupolar Dirac insulator and subsequently the mapping of the local pairing shown in Eq. (7) of the main text onto a time-reversal symmetry breaking, mixed parity octupolar pairing around a Fermi surface realized in the conduction band, for example. For concreteness, we focus near the $\Gamma=(0,0,0)$ point of the Brillouin zone and expand the tight-binding lattice Hamiltonian from Eq. (5) of the main text at low energies, yielding, the Nambu-doubled Hamiltonian of the form

$$H^{\rm low}_{\rm octu} = v(k_x\Gamma_1 + k_y\Gamma_2 + k_z\Gamma_3) + m\Gamma_4 + \Delta_1 d^{\rm low}_1(\boldsymbol{k})\Gamma_5 + \Delta_2 d^{\rm low}_2(\boldsymbol{k})\Gamma_6. \tag{S1}$$

The corresponding sixteen-dimensional mutually anticommuting Hermitian $\Gamma$ matrices are shown in Eq. (6) of the main text. In terms of the lattice parameters $v=ta$ bears the dimension of the Fermi velocity. Here we only kept the leading order term for the first-order Dirac mass, proportional to $\Gamma_4$. The form of the $d$-wave form factors $d^{\rm low}_1(\boldsymbol{k})$ and $d^{\rm low}_2(\boldsymbol{k})$ will be discussed in a moment.

The diagonalizing matrix that projects $H^{\rm low}_{\rm octu}$ onto the conduction band is a direct sum of the projectors onto the conduction band in the particle and hole subspaces. The particle block is obtained by columnwise arranging the eigenvector of $H^{\rm low}_{\rm octu}$ associated with the eigenvalue $+E(\boldsymbol{k})$ in the particle subspace, where

$$E(\boldsymbol{k}) = \sqrt{v^2\left(k_x^2+k_y^2+k_z^2\right) + m^2 + \left[d^{\rm low}_1(\boldsymbol{k})\right]^2 + \left[d^{\rm low}_2(\boldsymbol{k})\right]^2}. \tag{S2}$$

This eigenvalue is four-fold degenerate. Due to the Nambu doubling the conduction band energy is $-E(\boldsymbol{k})$ for holelike excitations. The diagonalizing matrix takes the form $U_{\rm diag} = U^{\rm particle}_{\rm diag} \oplus U^{\rm hole}_{\rm diag}$, where

$$\begin{aligned} U^{\rm particle}_{\rm diag} &= U\left(\boldsymbol{k}, d^{\rm low}_1(\boldsymbol{k}), d^{\rm low}_2(\boldsymbol{k})\right) = \frac{1}{\sqrt{2E(\boldsymbol{k})}} \begin{pmatrix} vk_x - ivk_y & vk_z - id^{\rm low}_1(\boldsymbol{k}) & 0 & m - id^{\rm low}_2(\boldsymbol{k}) \\ -vk_z - id^{\rm low}_1(\boldsymbol{k}) & vk_x + ivk_y & m - id^{\rm low}_2(\boldsymbol{k}) & 0 \\ 0 & -m - id^{\rm low}_2(\boldsymbol{k}) & vk_x - ivk_y & vk_z + id^{\rm low}_1(\boldsymbol{k}) \\ -m - id^{\rm low}_2(\boldsymbol{k}) & 0 & id^{\rm low}_1(\boldsymbol{k}) - vk_z & vk_x + ivk_y \\ 0 & 0 & 0 & 1 \\ 0 & 0 & 1 & 0 \\ 0 & 1 & 0 & 0 \\ 1 & 0 & 0 & 0 \end{pmatrix}, \\ U^{\rm hole}_{\rm diag} &= U\left(\boldsymbol{k}, -d^{\rm low}_1(\boldsymbol{k}), -d^{\rm low}_2(\boldsymbol{k})\right). \end{aligned} \tag{S3}$$

For the sake of notational compactness here we have taken $\Delta_j d^{\rm low}_j(\boldsymbol{k}) \to d^{\rm low}_j(\boldsymbol{k})$ for $j=1,2$. In terms of this diagonalizing matrix we then obtain the conduction-band projection of the Hamiltonian in Eq. (S1)

$$U^\dagger_{\rm diag} H^{\rm low}_{\rm octu} U_{\rm diag} = E(\boldsymbol{k})\left(\eta_3\, \mathbf{I}_{4\times 4}\right), \tag{S4}$$

where $\mathbf{I}_{4\times 4}$ is a four-dimensional identity matrix and the Pauli matrix $\eta_3$ operates on the Nambu or particle-hole index. Therefore, in the presence of a finite chemical doping the normal state band dispersion of the conduction band around the Fermi surface reads

$$H_0^{\rm FS} = (E(\boldsymbol{k}) - \mu)\, \eta_3 \tau_0 \beta_0 \approx \left( \frac{k^2}{2m} - \mu_* \right) \Gamma_{300} + \mathcal{O}(k^4), \tag{S5}$$

where $\Gamma_{300} = \eta_3 \tau_0 \beta_0$. While arriving at the final expression we neglect the terms arising from $\Delta_1$ and $\Delta_2$, assuming that $\Delta_1, \Delta_2 \ll m$. Here we perform a large mass expansion, and $\mu_* = \mu - m$ is the effective chemical potential measured from the bottom of the conduction band.

We now apply the diagonalizing operator on the local pairing shown in Eq. (7) of the main text. In the close vicinity to the Fermi surface, after the projection onto the conduction band, this local pairing for the U(1) superconducting phase $\phi = 0$ assumes the following form

$$\begin{aligned} H^{\rm proj}_{\rm local} &= \Delta \begin{pmatrix} 0_{4\times 4} & \left[U^{\rm particle}_{\rm diag}\right]^\dagger (\beta_1 \tau_1 \sigma_0)\, U^{\rm hole}_{\rm diag} \\ \left[U^{\rm hole}_{\rm diag}\right]^\dagger (\beta_1 \tau_1 \sigma_0)\, U^{\rm particle}_{\rm diag} & 0_{4\times 4} \end{pmatrix} \\ &= \frac{\Delta}{m} \left[ \frac{t}{k_{_F}} \left( k_x \Gamma_{101} - k_y \Gamma_{102} - k_z \Gamma_{103} \right) + \Delta_1 d_1^{\rm low}(\boldsymbol{k}) \Gamma_{230} + \Delta_2 d_2^{\rm low}(\boldsymbol{k}) \Gamma_{210} \right], \end{aligned} \tag{S6}$$

where the Fermi momentum $k_{_F} = a^{-1}$. While arriving at the final expression we have assumed $m \gg v|\boldsymbol{k}|, \Delta_1, \Delta_2$ which is justified in the large mass limit. Notice that all the five matrices appearing in $H^{\rm proj}_{\rm local}$ are mutually anticommuting, and also anticommute with $H_0^{\rm FS}$. Finally, performing a *global* unitary rotation by the unitary operator

$$U = \begin{pmatrix} \frac{1}{\sqrt{2}} & 0 & -\frac{i}{\sqrt{2}} & 0 & 0 & 0 & 0 & 0 \\ 0 & \frac{1}{\sqrt{2}} & 0 & -\frac{i}{\sqrt{2}} & 0 & 0 & 0 & 0 \\ \frac{1}{\sqrt{2}} & 0 & \frac{i}{\sqrt{2}} & 0 & 0 & 0 & 0 & 0 \\ 0 & \frac{1}{\sqrt{2}} & 0 & \frac{i}{\sqrt{2}} & 0 & 0 & 0 & 0 \\ 0 & 0 & 0 & 0 & \frac{1}{\sqrt{2}} & 0 & \frac{i}{\sqrt{2}} & 0 \\ 0 & 0 & 0 & 0 & 0 & \frac{1}{\sqrt{2}} & 0 & \frac{i}{\sqrt{2}} \\ 0 & 0 & 0 & 0 & \frac{1}{\sqrt{2}} & 0 & -\frac{i}{\sqrt{2}} & 0 \\ 0 & 0 & 0 & 0 & 0 & \frac{1}{\sqrt{2}} & 0 & -\frac{i}{\sqrt{2}} \end{pmatrix}, \tag{S7}$$

we arrive at the total effective single particle Hamiltonian in the vicinity of the Fermi surface in the presence of the local pairing shown in Eq. (7) of the main text

$$\begin{aligned} \left[U_{\rm diag}\right]^\dagger \left( H_0^{\rm FS} + H^{\rm proj}_{\rm local} \right) U_{\rm diag} = \left( \frac{k^2}{2m} - \mu_* \right) \Gamma_{300} + \Delta_p \left[ \Gamma_{131} \frac{k_x}{k_{_F}} + \Gamma_{132} \frac{k_y}{k_{_F}} + \Gamma_{133} \frac{k_z}{k_{_F}} \right] \\ + \Delta_1 d_1^{\rm low}(\boldsymbol{k}) \Gamma_{110} + \Delta_2 d_2^{\rm low}(\boldsymbol{k}) \Gamma_{200}. \end{aligned} \tag{S8}$$

This Hamiltonian is identical to the one shown in Eq. (1) of the main text, with $\Delta_p = \Delta t/m$, $\Delta \Delta_1/m \to \Delta_1$, $\Delta \Delta_2/m \to \Delta_2$, $m_* \to m$, $\mu \to \mu_*$, and $\Delta_s = 0$.

We now focus on the $d$-wave form factors. We always take $d_2^{\rm low}(\boldsymbol{k}) = (2k_z^2 - k_x^2 - k_y^2)/(2k_{_F}^2)$ in Eq. (S1), obtained as low energy expansion of the lattice term $-[2\cos(k_z a) - \cos(k_x a) - \cos(k_y a)]$ near the $\Gamma$ point, as discussed in the main manuscript, with $k_{_F} = a^{-1}$. For intrinsic third-order topological superconductor, $d_1^{\rm low}(\boldsymbol{k}) = \sqrt{3}(k_x^2 - k_y^2)/(2k_{_F}^2)$, obtained by expanding $-\sqrt{3}[\cos(k_x a) - \cos(k_y a)]$ around the $\Gamma$ point. Finally, for the extrinsic third-order topological superconductor $d_1^{\rm low}(\boldsymbol{k}) = \sqrt{3}(k_x k_y)/k_{_F}^2$, which can be obtained by expanding $\sqrt{3}\sin(k_x a)\sin(k_y a)$ around the $\Gamma$ point. Therefore, the same local pairing, shown in Eq. (7) of the main text, yields the intrinsic or extrinsic third-order topological superconductor in a doped octupolar Dirac insulator when projected onto the Fermi surface, depending on the form of the Wilson-Dirac mass form factor $d_1(\boldsymbol{k})$. Here we show the band projection of this pairing on the conduction band. Identical conclusion holds when we project the pairing onto the valence band.

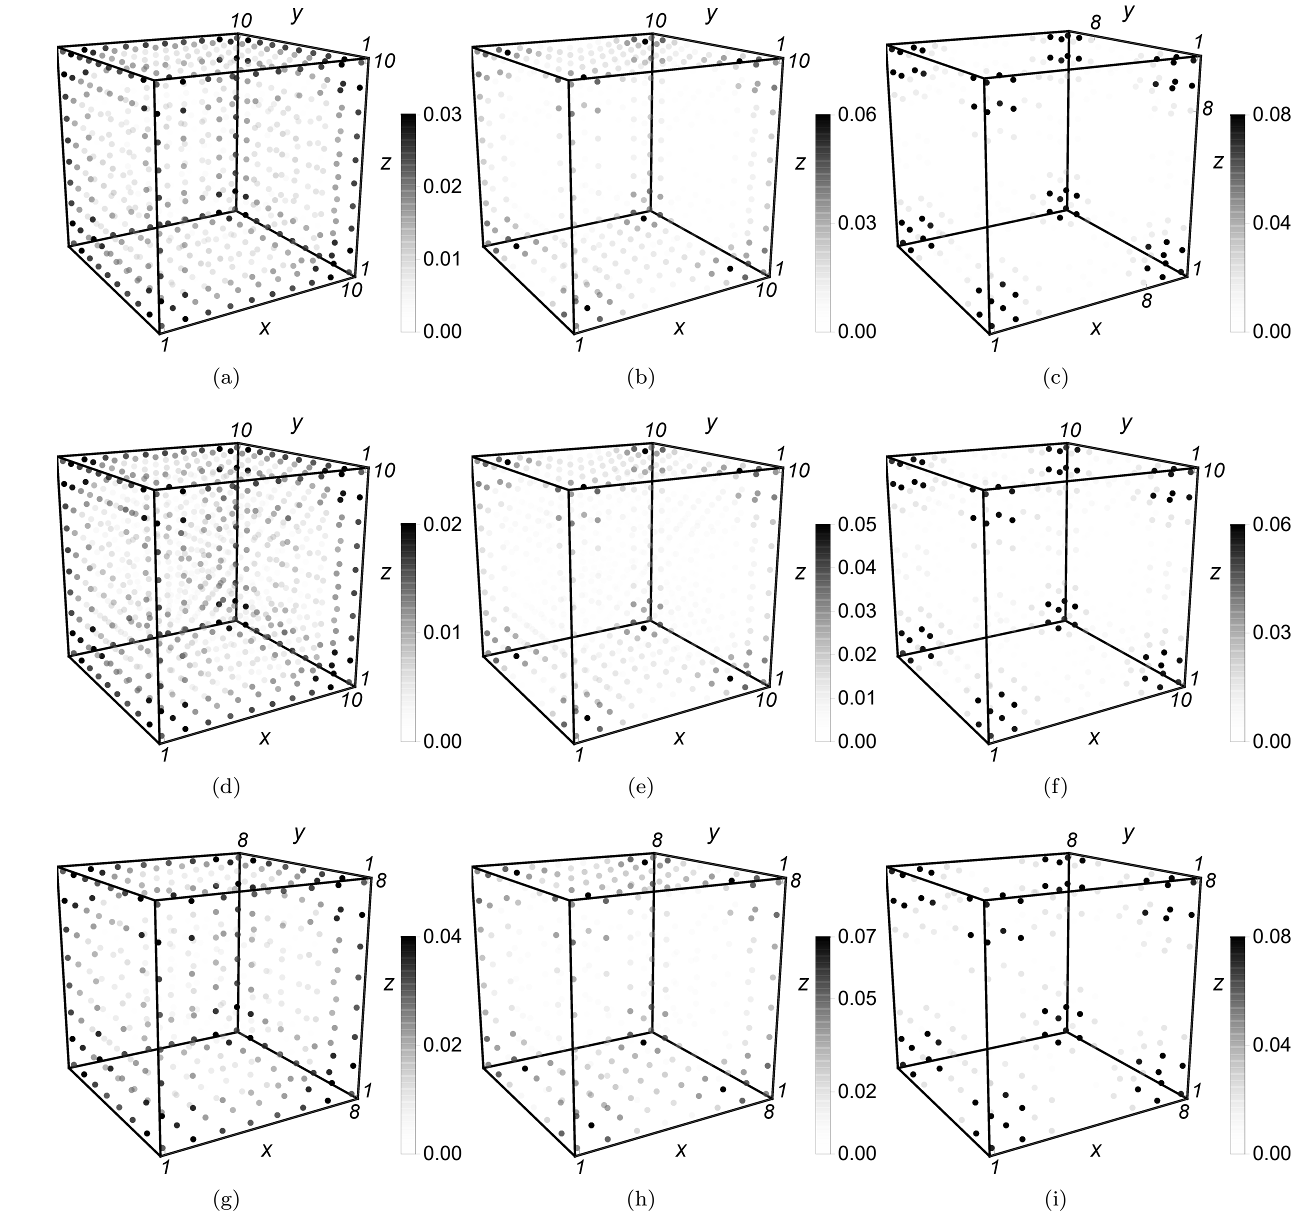


FIG. S1: Local density of states (LDOS) for *gapless* (a) surface states of an isotropic (first-order) $p$-wave pairing, (b) $z$ directional hinge modes and $xy$ surface modes of a second-order topological superconductor (TSC) and (c) corner modes of a third order TSC. In (a) we set $t_1 = t_0 = m_0/2 = 1$ and $\Delta_1 = \Delta_2 = \Delta_s = 0$ in Eq. (5) of the main text, while in (b) $\Delta_1 = 1$, but $\Delta_2 = 0$, and in (c) $\Delta_1 = \Delta_2 = 1$. Panels (d), (e) and (f) are analogous to (a), (b) and (c), respectively, but in the presence of a small $s$-wave component $\Delta_s = 0.5$. For these two rows all pairings are realized around a Fermi surface near the $\Gamma = (0, 0, 0)$ point of the Brillouin zone, and $\Gamma$ matrices in Eq. (5) are eight-dimensional. LDOS associated with the boundary mode for the local pairing shown in Eq. (7) of the main text, in a trivial octupolar Dirac insulator [with sixteen-component $\Gamma$ matrices in Eq. (6)] for $t_1 = t_0 = -m_0/2 = 1$, $\Delta_s = \mu = 0$ and (g) $\Delta_1 = \Delta_2 = 0$, (h) $\Delta_1 = 1$, $\Delta_2 = 0$ and (i) $\Delta_1 = \Delta_2 = 1$. Thus same local pairing yields (g) first-order, (h) second-order and (i) third-order TSC. Here all the realizations of third-order TSC are intrinsic, as we set $d_1^{\rm lat}(\boldsymbol{k}) = \cos(k_x a) - \cos(k_y a)$ in the lattice model. We always take $d_2^{\rm lat}(\boldsymbol{k}) = 2\cos(k_z a) - \cos(k_x a) - \cos(k_y a)$.

## S2. ADDITIONAL NUMERICAL RESULTS: EVOLUTION OF TOPOLOGICAL SUPERCONDUCTOR

In this section, we briefly outline the extensive numerical results presented in Figs. S1 and S2. These two figures show the evolution of topological superconductors, from the first-order to second-order to the third-order. Namely

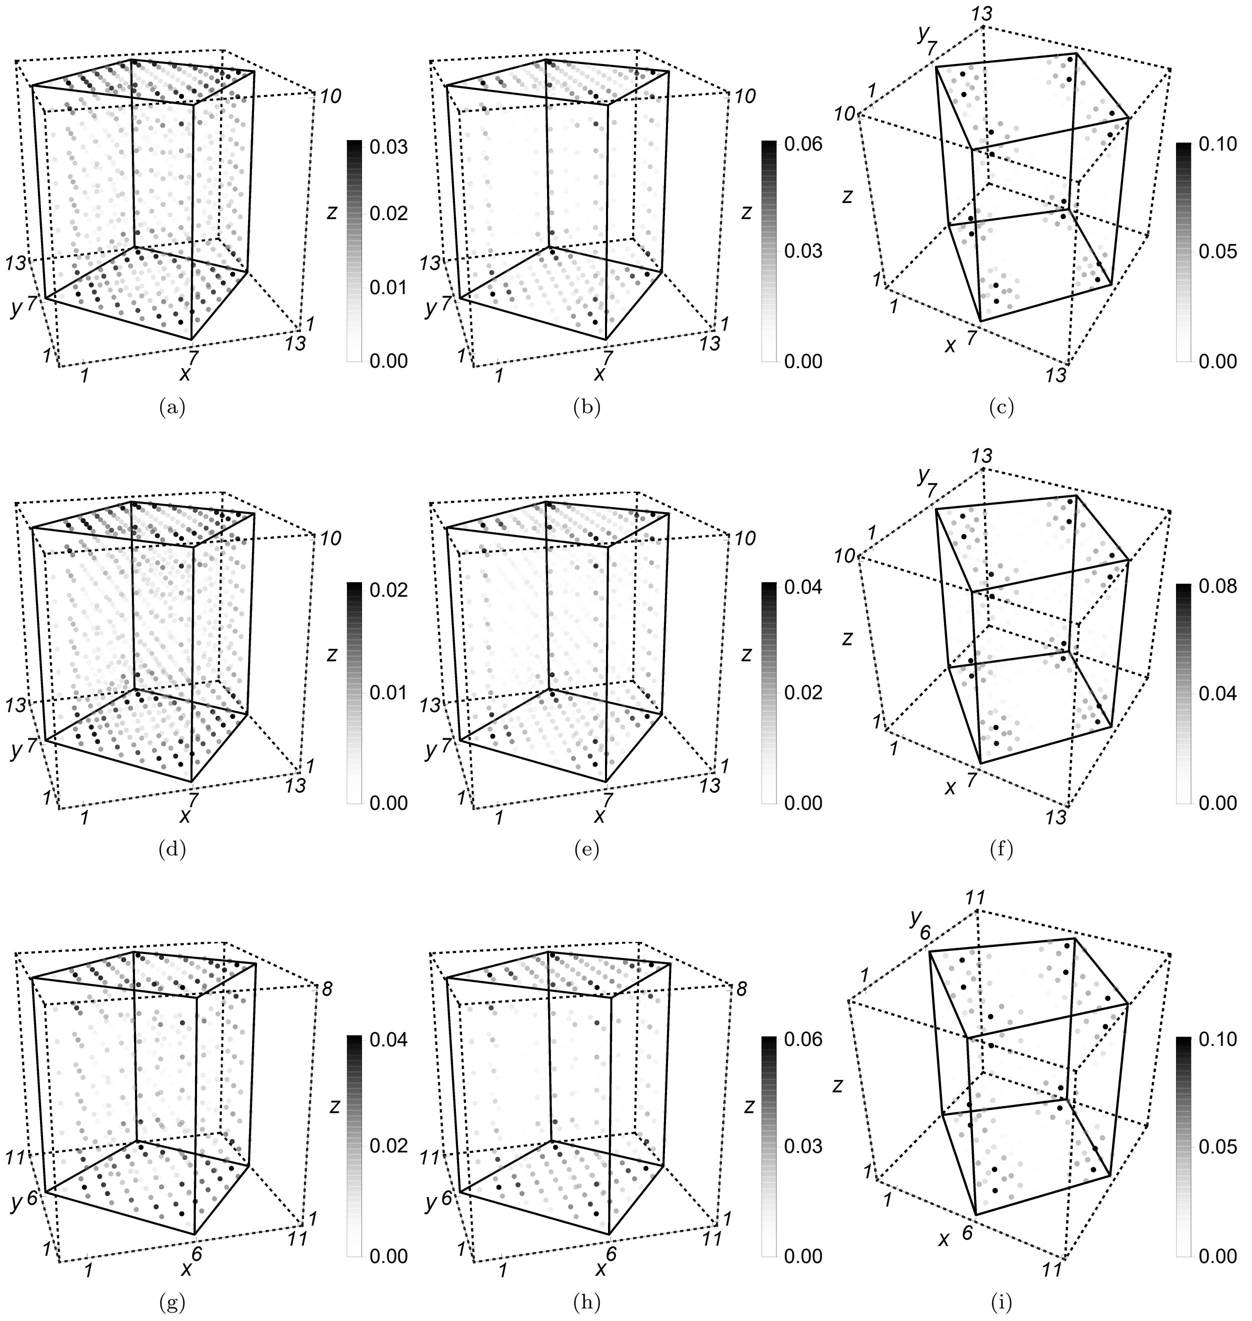


FIG. S2: All the panels are identical to the corresponding to ones in Fig. S1. We keep all the parameter values identical, but take $d_1^{\rm lat} = \sin(k_x a)\sin(k_y a)$ in the lattice model. Therefore, the third-order topological superconductors (third column of each row) are extrinsic in nature. The crystal cut of the cubic lattice is identical to the one shown in Fig. 2 of the main text.

the third-order superconductor supporting corner localized Majorana modes shown in these two figures are intrinsic and extrinsic, respectively. The crystals cuts of the cubic lattice in these two figures are identical to the ones shown in Figs. 1 and 2 of the main text, respectively. In both the figures the first column shows the surface state of a first-order topological superconductor, the second column shows gapless hinge modes along the $z$ direction and surface modes on the $xy$ planes of second-order topological superconductors, and the third column shows corner localized Majorana modes in suitably cleaved cubic crystals. The rest of the details are presented in the captions of these two figures.

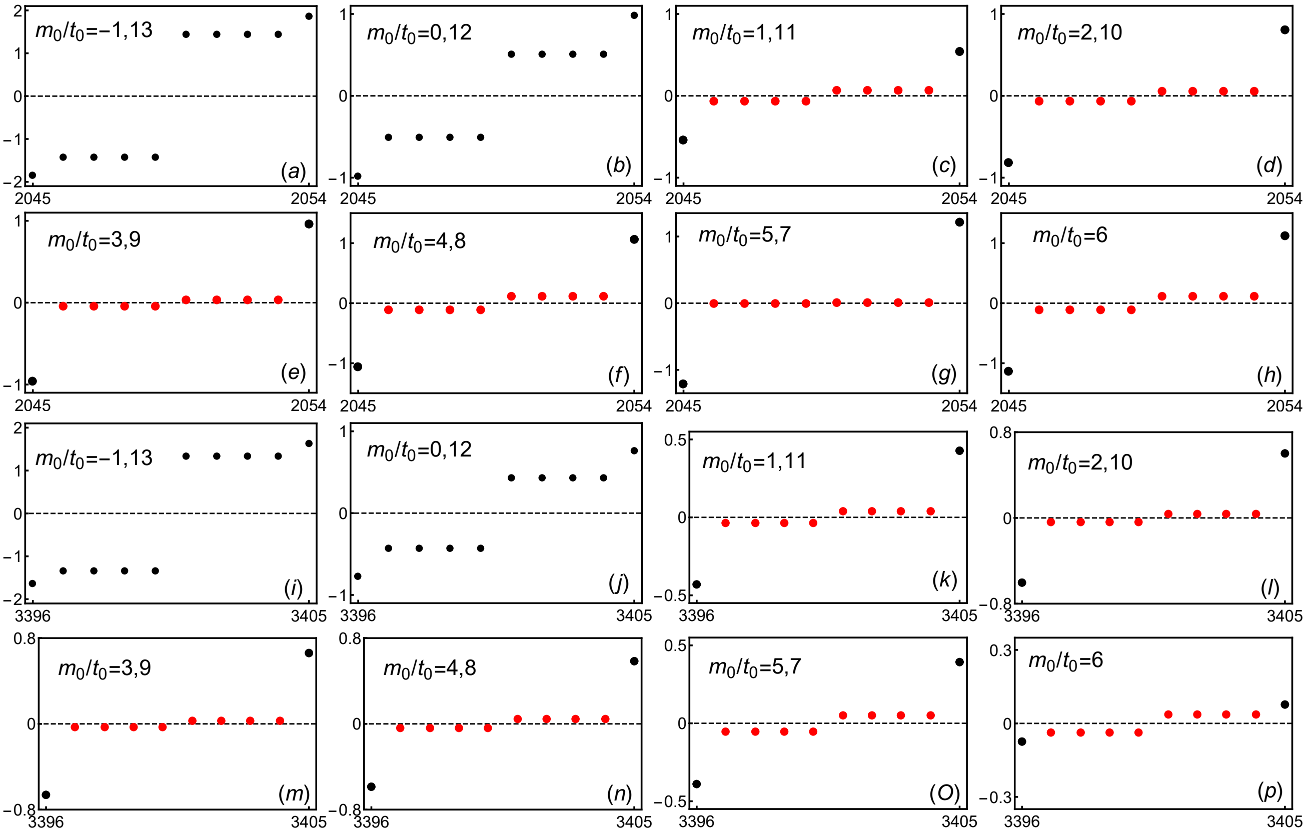


FIG. S3: Energy spectra for ten closest to zero energy states for intrinsic [panels $(a)$-$(h)$] and extrinsic [panels $(i)$-$(p)$] octupolar pairings on cubic lattice with open boundary condition, cleaved following the prescription from Fig. 1(b) and Fig. 2(b) of the main text, respectively, realized for the lattice regularized BdG Hamiltonian, shown in Eqs. (1) and (6) of the main text. Throughout we set $t_1 = t_0 = \Delta_1 = \Delta_2 = 1.0$ and $\Delta_s = 0$. The values for $m_0/t_0$ are quoted in each panel. The corner modes, when exist, are shown in red, while the closest to zero energy bulk states are shown in black. The corner modes are placed very close to, but not precisely at zero energy due to finite system size. Therefore, within the parameter regime $0 < m_0/t_0 < 12$ we find topological octupolar pairing, while for $m_0/t_0 < 0$ and $m_0/t_0 > 12$ the paired states are topologically trivial. Here we do not explicitly show the LDOS associated with the corner modes to avoid repetition. But, they show qualitatively similar features as in Fig. 1(b) and Fig. 2(b) of the main text respectively for intrinsic and extrinsic octupolar pairings. In panels $(a)$-$(h)$ the linear dimension of the system is $L = 8$ in each direction. In panels $(i)$-$(p)$, the linear dimension of the system in the $x$, $y$ and $z$ directions are $L_x = 13$, $L_y = 13$ and $L_z = 10$, respectively. In all the panels the vertical and horizontal axes display the energy eigenvalues and their indices, respectively, and we implement open boundary condition.

## S3. PARAMETER REGIME FOR OCTUPOLAR TOPOLOGICAL SUPERCONDUCTOR

In the main manuscript, we claimed that for the lattice model shown in Eq. (6) with eight-component Hermitian $\Gamma$ matrices, third-order octupolar topological pairings (both intrinsic and extrinsic) are realized in the tight binding parameter regime $0 < m_0/t_0 < 12$ when $t_1 = 1$, but $\Delta_1$ and $\Delta_2$ taking arbitrary, but finite values. In this entire parameter regime the paired states accommodate eight near (due to finite system size) zero energy modes, which are well separated (by a finite energy gap) from the rest of the bulk states. On the other hand, in the parameter regimes $m_0/t_0 < 0$ and $m_0/t_0 > 12$ the pairied states are topologically trivial and do not support any near zero energy corner modes. These outcomes are summarized in Fig. S3 for both intrinsic [panels $(a)$-$(h)$] and extrinsic [panels $(i)$-$(p)$] octupolar pairings in open cubic systems. We show eight corner modes (when exist) in red, while the closest to zero energy bulk states are shown in black. All the red states show sharp corner localization for both intrinsic and extrinsic pairings, when the cubic crystal is cleaved following the prescription respectively shown in Fig. 1(b) and Fig. 2(b) of the main text and we impose open boundary condition. To avoid repetition, here we do not show the local density of states explicitly for the corner modes.

| Pairing | | Dirac kinetic term | | | First-order Dirac mass | Higher-order Dirac mass | | TSC (?) |
|---|---|---|---|---|---|---|---|---|
| Amplitude | Γ-matrix | $\Gamma_{3111}$ | $\Gamma_{3112}$ | $\Gamma_{3113}$ | $\Gamma_{3130}$ | $\Gamma_{0120}$ | $\Gamma_{0200}$ | |
| $\Delta^j_A$ | $\Gamma_{\alpha 20j}$ | $(+,-,-)$ | $(-,+,-)$ | $(-,-,+)$ | $(+,+,+)$ | $(-,-,-)$ | $(+,+,+)$ | |
| $\Delta^j_B$ | $\Gamma_{\alpha 21j}$ | $(+,-,-)$ | $(-,+,-)$ | $(-,-,+)$ | $(-,-,-)$ | $(+,+,+)$ | $(+,+,+)$ | × |
| $\Delta^j_C$ | $\Gamma_{\alpha 23j}$ | $(-,+,+)$ | $(+,-,+)$ | $(+,+,-)$ | $(+,+,+)$ | $(+,+,+)$ | $(+,+,+)$ | |
| $\Delta_D$ | $\Gamma_{\alpha 220}$ | $-$ | $-$ | $-$ | $-$ | $-$ | $+$ | × |
| $\Delta^0_E$ | $\Gamma_{\alpha 000}$ | $-$ | $-$ | $-$ | $-$ | $+$ | $+$ | × |
| $\Delta^1_E$ | $\Gamma_{\alpha 010}$ | $-$ | $-$ | $-$ | $+$ | $-$ | $+$ | |
| $\Delta^3_E$ | $\Gamma_{\alpha 030}$ | $+$ | $+$ | $+$ | $-$ | $-$ | $+$ | × |
| $\Delta^j_F$ | $\Gamma_{\alpha 02j}$ | $(+,-,-)$ | $(-,+,-)$ | $(-,-,+)$ | $(+,+,+)$ | $(+,+,+)$ | $(+,+,+)$ | |
| $\Delta^0_G$ | $\Gamma_{\alpha 100}$ | $-$ | $-$ | $-$ | $-$ | $+$ | $-$ | × |
| $\Delta^1_G$ | $\Gamma_{\alpha 110}$ | $-$ | $-$ | $-$ | $+$ | $-$ | $-$ | TOTSC |
| $\Delta^3_G$ | $\Gamma_{\alpha 130}$ | $+$ | $+$ | $+$ | $-$ | $-$ | $-$ | × |
| $\Delta^j_H$ | $\Gamma_{\alpha 12j}$ | $(+,-,-)$ | $(-,+,-)$ | $(-,-,+)$ | $(+,+,+)$ | $(+,+,+)$ | $(-,-,-)$ | |
| $\Delta^0_I$ | $\Gamma_{\alpha 300}$ | $+$ | $+$ | $+$ | $+$ | $-$ | $-$ | |
| $\Delta^1_I$ | $\Gamma_{\alpha 310}$ | $+$ | $+$ | $+$ | $-$ | $+$ | $-$ | × |
| $\Delta^3_I$ | $\Gamma_{\alpha 330}$ | $-$ | $-$ | $-$ | $+$ | $+$ | $-$ | |
| $\Delta^j_J$ | $\Gamma_{\alpha 32j}$ | $(-,+,+)$ | $(+,-,+)$ | $(+,+,-)$ | $(-,-,-)$ | $(-,-,-)$ | $(-,-,-)$ | × |

TABLE I: Classification of all the local pairing terms in the octupolar Dirac insulator. All possible 28 pairing terms are grouped into 16 channels according to their symmetries. The label + (−) indicates that the pairing Γ-matrix commutes (anticommutes) with the corresponding Dirac kinetic term, the first-order and the higher-order Dirac masses. In the last column, × denotes a pairing that cannot realize a topological superconductor because it anticommutes with the uniform first-order Dirac mass, which fully gaps out any surface states (if exist). Only the pairing represented by the matrix $\Gamma_{\alpha 110}$ can realize a third-order topological superconductor (TOTSC), as it fully anticommutes with Dirac kinetic term and the higher-order Dirac masses, while commutes with the first-order Dirac mass. The index $j = 1, 2, 3$ denotes the components of a triplet pairing, while $\alpha = 1, 2$ corresponds to the U(1) phase redundancy when defining a superconducting order parameter.

## S4. COMPETITION AMONG LOCAL PAIRINGS IN OCTUPOLAR DIRAC INSULATOR

In this section, we compute the competition among all 28 local pairings in an octupolar Dirac insulator. First we identify that these pairings can be grouped into eight triplet and eight singlet channels, according to the algebraic properties of the associated pairing matrices with the ones appearing in the massive Dirac Hamiltonian, given by

$$H^{\rm lat}_{\rm octu} = t_1 \sum_{j=1,2,3} \sin(k_j a)\Gamma_{311j} + \Gamma_{3130}\, m^{\rm lat}_1(\mathbf{k}) - \Delta_1\, \Gamma_{0120}\sqrt{3}\, d^{\rm lat}_1(\boldsymbol{k}) - \Delta_2\, \Gamma_{0200}\, d^{\rm lat}_2(\boldsymbol{k}), \tag{S9}$$

where

$$\begin{aligned} m^{\rm lat}_1(\mathbf{k}) &= m_0 - 6t_0 + 2t_0 \sum_{j=1,2,3} \cos(k_j a), \quad d^{\rm lat}_1(\boldsymbol{k}) = \cos(k_x a) - \cos(k_y a) \ \text{ or } \ \sin(k_x a)\sin(k_y a), \\ d^{\rm lat}_2(\boldsymbol{k}) &= 2\cos(k_z a) - \cos(k_x a) - \cos(k_y a). \end{aligned} \tag{S10}$$

Two functional forms of $d^{\rm lat}_1(\boldsymbol{k})$ respectively correspond to intrinsic or extrinsic octupolar Dirac insulator. Hereafter, we set the lattice spacing $a = 1$. The effective single-particle Hamiltonian in the presence of all the local pairings after grouping them according to their symmetry properties assumes the following form

$$\begin{aligned} H_{\rm pair} = &\sum_{j=1,2,3} \Delta^j_A \Gamma_{\alpha 20j} + \sum_{j=1,2,3} \Delta^j_B \Gamma_{\alpha 21j} + \sum_{j=1,2,3} \Delta^j_C \Gamma_{\alpha 23j} + \Delta_D \Gamma_{\alpha 220} + \Delta^0_E \Gamma_{\alpha 000} + \Delta^1_E \Gamma_{\alpha 010} + \Delta^3_E \Gamma_{\alpha 030} \\ &+ \sum_{j=1,2,3} \Delta^j_F \Gamma_{\alpha 02j} + \Delta^0_G \Gamma_{\alpha 100} + \Delta^1_G \Gamma_{\alpha 110} + \Delta^3_G \Gamma_{\alpha 130} + \sum_{j=1,2,3} \Delta^j_H \Gamma_{\alpha 12j} + \Delta^0_I \Gamma_{\alpha 300} + \Delta^1_I \Gamma_{\alpha 310} \\ &+ \Delta^3_I \Gamma_{\alpha 330} + \sum_{j=1,2,3} \Delta^j_J \Gamma_{\alpha 32j}. \end{aligned} \tag{S11}$$

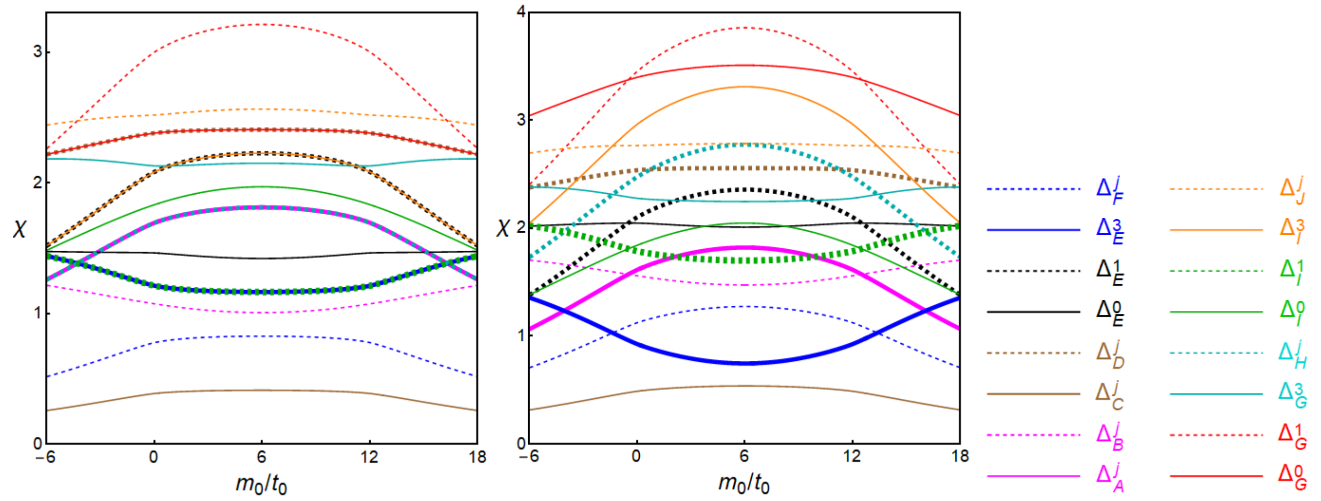


(a) (b) (c)

FIG. S4: Bare mean field susceptibility ($\chi$), defined in Eq. (S12), for all the local pairings, shown in Eq. (S11), in an octupolar Dirac insulator, described by the Hamiltonian defined through Eqs. (S9) and (S10), over a wide range of $m_0/t_0$ covering both topological and trivial insulating phases in the normal state, for $t_1 = \Delta_1 = \Delta_2 = 1$. In panel (a) the third-order or octupolar pairing (red dashed line) is intrinsic, while that in (b) is extrinsic in nature. The susceptibility of the paring channels are color coded, see panel (c). This computation shows that both intrinsic and extrinsic octupolar pairings are energetically most favored over a wide range of $m_0/t_0$, indicated by their largest susceptibilities among all the symmetry allowed local pairing channels. Furthermore, among all the candidate topological paired states (commuting with first-order Dirac mass, see Table I) $\Delta_A^j$ (solid magenta), $\Delta_C^j$ (solid brown), $\Delta_E^1$ (dashed black), $\Delta_F^j$ (dashed blue), $\Delta_G^1$ (dashed red), $\Delta_H^j$ (dashed cyan), $\Delta_I^0$ (dashed green), $\Delta_I^3$ (solid orange), the local octupolar pairing ($\Delta_G^1$) yielding TOTSC always possesses the largest susceptibility for any $m_0/t_0$.

See Table I. Here sixteen-dimensional Hermitian $\Gamma$ matrices are defined as $\Gamma_{\mu\nu\rho\lambda} = \eta_\mu \beta_\nu \tau_\rho \sigma_\lambda$ with $\mu, \nu, \rho, \lambda = 0, \cdots, 3$. Four sets of the Pauli matrices $\{\eta_\mu\}$, $\{\beta_\nu\}$, $\{\tau_\rho\}$ and $\{\sigma_\lambda\}$ respectively operate on the Nambu or particle-hole, sublattice, parity and spin indices. In the pairing matrices $\alpha = 1$ or $2$ manifesting the U(1) gauge redundancy in defining the superconducting phase. However, the following conclusions are completely insensitive to the choice of $\alpha$ and for the sake of concreteness we fix $\alpha = 1$ for the rest of the discussion.

Valuable information on the competition among superconducting orders can be gained by computing and comparing their bare mean-field susceptibilities at zero external momentum and frequency. For example, the bare mean field susceptibility ($\chi$) for a superconducting order appearing with a sixteen-dimensional Hermitian matrix $M$ is given by

$$\chi = -\int_{-\pi}^{\pi} \frac{dk_x}{2\pi} \int_{-\pi}^{\pi} \frac{dk_y}{2\pi} \int_{-\pi}^{\pi} \frac{dk_z}{2\pi} \int_{-\infty}^{\infty} \frac{d\omega}{2\pi} \, \mathrm{Tr}\left[ G(i\omega, \boldsymbol{k}) M G(i\omega, \boldsymbol{k}) M \right], \tag{S12}$$

where $\omega$ is the fermionic Matsubara frequency and $G(i\omega, \boldsymbol{k}) = (i\omega - H^{\rm lat}_{\rm octu})^{-1}$ is the fermionic Green's function. The integration over momentum is performed over the entire first Brillouine zone. The scaling of the susceptibility for all sixteen symmetry allowed pairing channels as a function of $m_0/t_0$ are shown in Fig. S4.

The bare mean-field susceptibility $\chi$ provides the following information. (1) Inverse of $\chi$ is proportional to the requisite strength for critical interaction strength ($g_\star$) for the nucleation of the corresponding pairing order, i.e. $g_\star \propto \chi^{-1}$, which is always finite in any Dirac system (gapless or gapped) due to the vanishing density of states. (2) For energetic comparison: if we set the amplitudes of all pairing orders equal, then the ground state condensation energy is proportional to $\chi$ up to an overall unimportant shift. Fig. S4 shows that the candidate pairing order yielding an octupolar third-order topological superconductor possesses *largest* susceptibility over a wide range of the parameter $m_0/t_0$, which includes both topological and trivial parent Dirac insulating phase. Hence, the computation of the bare mean field susceptibility immediately suggest that the onset of the proposed third-order or octupolar paired state [$\Delta_G^1$ in Eq. (S11) or $H_{\rm octu}$ in Eq. (7) of the main text] requires minimal critical coupling and it also provides maximal gain of condensation energy among all symmetry allowed local superconducting states over a wide parameter range. Therefore, in a conducive environment, when electron-electron interactions develop a strong attractive component $\Delta_G^1$ pairing is expected to be energetically favored, as announced toward the end of the main manuscript.
